# Supplementary material for: Independent Distribution Regularization for Private Graph Embedding
Source: arXiv:2308.08360 source file (2023-08-16)
Supplement: Supplementary file 1 [file appendix.tex]

\appendix
